# Supplementary material for: Iterative Rule Extension for Logic Analysis of Data: an MILP-based heuristic to derive interpretable binary classification from large datasets
Source: arXiv:2110.13664 source file (2021-10-25)
Supplement: Supplementary file 1 [file IRELAND_appendices.pdf]

# Appendix to "Iterative Rule Extension for Logic Analysis of Data: an MILP-based heuristic to derive interpretable binary classification from large datasets"

Marleen Balvert

## A Lemmas and proofs

**Lemma 1.** *Given a set of AND clauses $\mathcal{K}$, then for all $k \in \mathcal{K}$ and $n \in \mathcal{N}$ let $t_{nk} = 1$ if and only if sample $n$ satisfies clause $k$. Define:*

- $P1 = \{\hat{y} \in [0,1]^{\mathcal{N}} : (1a)$ *and* $(1b)$ *are satisfied;*
- $P2 = \{\hat{y} \in [0,1]^{\mathcal{N}} : (2a)$ *and* $(2b)$ *are satisfied.*

*Then $P2 \subseteq P1$.*

*Proof.* First note that equations (1a) and (2a) are identical. Second, (2b) $\Rightarrow$ (1b) is trivial. In order to see that (1b) does not imply (2b), consider the following example. Suppose that $\mathcal{K} = \{1, 2\}$, $t_{n1}$ and $t_{n2} = 0$ for some $n \in \mathcal{N}_0$. Then constraint (2b) enforces $\hat{y}_n = 1$, while constraint (1b) only requires $\hat{y}_n \geq 0.5$. $\square$

**Lemma 2.** *Define:*

- $P3 = \{t \in [0,1]^{N \times K},\ s \in [0,1]^{J \times K}$ : *(3a) and (3b) are satisfied* $\forall j \in \mathcal{J}, \forall n \in \mathcal{N}, \forall k \in \mathcal{K}\}$;
- $P4 = \{t \in [0,1]^{N \times K},\ s \in [0,1]^{J \times K}$ : *(4a) and (4b) are satisfied* $\forall j \in \mathcal{J}, \forall n \in \mathcal{N}, \forall k \in \mathcal{K}\}$.

*Then $P4 \subseteq P3$.*

*Proof.* Since (3b) and (4b) are identical, it suffices to show that (4a) $\Rightarrow$ (3a), but (3a) $\Rightarrow$ (4a) does not hold.
<u>(4a) $\Rightarrow$ (3a)</u>

$$\begin{aligned}
& t_{nk} - (X_{nj} - 1)s_{kj} && \leq 1 \quad \forall j \in \mathcal{J} \\
\Leftrightarrow\ & t_{nk} - (X_{nj} - 1)s_{kj} - X_{nj} + (X_{nj} - 1) && \leq 0 \quad \forall j \in \mathcal{J} \\
\Leftrightarrow\ & t_{nk} + (1 - X_{nj})(1 - s_{kj}) + X_{nj} && \leq 0 \quad \forall j \in \mathcal{J} \\
\Rightarrow\ & J \cdot t_{nk} + \sum_{j \in \mathcal{J}} (1 - X_{nj})(1 - s_{kj}) + \sum_{j \in \mathcal{J}} X_{nj} && \leq 0
\end{aligned}$$

(3a) does not imply (4a) Consider the following example. Let $\mathcal{J} = \{1, 2\}$, $w_{k1} = \frac{1}{4}$, $s_{k2} = \frac{3}{4}$ for some $k \in \{1, ..., K\}$, $X_{n1} = 0$ and $X_{n2} = 0$ for some $n \in \mathcal{N}$. Then (3a) implies:

$$2 \cdot t_{nk} - \frac{1}{4} + \frac{3}{4} \leq 0 \Leftrightarrow t_{nk} \leq \frac{1}{2},$$

while this is not feasible with respect to constraint (4a):

$$\begin{cases} t_{nk} + \frac{1}{4} \leq 1 \\ t_{nk} + \frac{3}{4} \leq 1 \end{cases} \Leftrightarrow t_{nk} \leq \frac{1}{4}.$$

□

# B Effect of data sizes on runtime of $(BP1)$

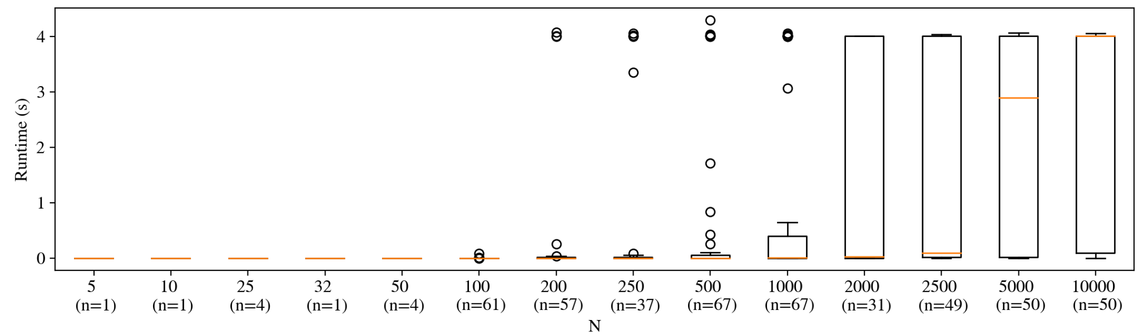


(a)

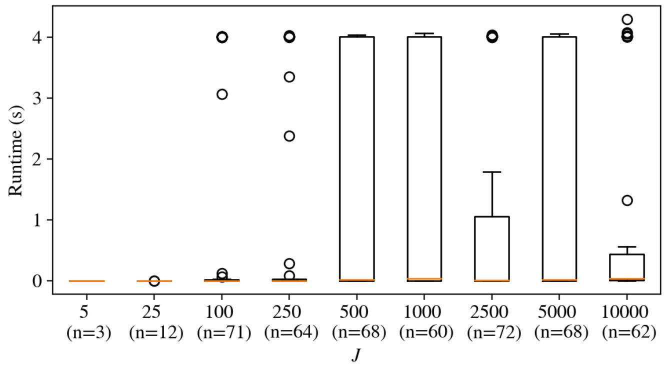


(b)

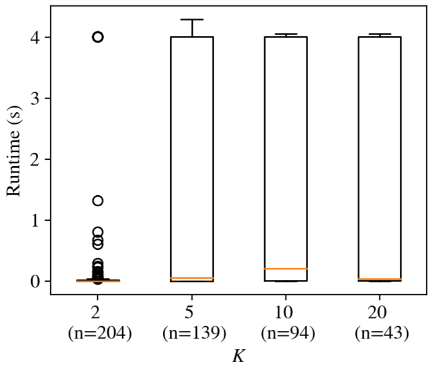


(c)

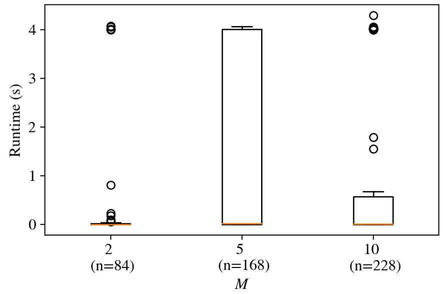


(d)

Figure 1: Runtimes obtained with $(BP1)$ for various no noise datasets, aggregated by (a) the number of samples $N$, (b) the number of features $J$, (c) the number of AND clauses $K$ and (d) the maximum number of features per clause $M$. The figures show that $N$ has a major impact on the performance of $(BP1)$. $J$ and $K$ influence its performance as well, while $M$ does not seem to be related to model performance.
